# Supplementary material for: Hierarchical surrogate-based Approximate Bayesian Computation for an electric motor test bench
Source: arXiv:2106.09597 source file (2021-06-17)
Supplement: Supplementary file 1 [file appendix.tex]

\section{Additional numerical results}
